# Supplementary material for: Topic-wise Exploration of the Telegram Group-verse
Source: arXiv:2409.02525 source file (2025-03-17)
Supplement: Supplementary file 1 [file 9999-appendix-reviews.tex]

\section{TheWebConf reviews}

\subsection{Reviewer uQQ5}

\subsubsection{Review}

This paper collects several posts from active groups on Telegram in April 2024 and then studies what types of non-text media are used in each post stratified by the topic of the post.

\textbf{Strengths:}

\begin{enumerate}
    \item I haven’t seen too much work using telegram, and exploring a new site is interesting
    \item The idea of sampling groups off of the TGStat website was interesting, and releasing your crawler and dataset will be very useful
    \item The main takeaways at the end of each section are really useful
    \item The results are laid out cleanly and systematically
\end{enumerate}

\textbf{Weaknesses:}

\begin{enumerate}
    \item It’s not clear what you mean by “user activity patterns” in line 45. Could you be more specific, since it’s important to understand the study hypothesis?
    \item Is the goal of the paper to describe differences between the types of non-text engagement across topics? Or is there a hypothesis you’re testing? In the former case, you could you reword the hypothesis to frame it as a descriptive aim? In the latter case, you would need to use statistical tests to show that there are significant differences, adjust for multiple hypothesis corrections, etc.
    \item Can you say more about how we should interpret the sample? I assume it’s not truly a random sample of Telegraph, but do you have intuition about the types of posts that would and wouldn’t be included in the sample? I think it’s really important to be clear about this because it’s not clear that your results generalize to all of telegraph, just to the types of posts that were in your sample.
    \item A big focus of the paper is to compare rates of various non-text engagements in the data by topic. However there is little to no discussion about the implications or importance of these findings; specifically, why is it useful to know different media of engagement by topic?
    \item It’s great that you verified TGStat’s topic labels, but were you able to check their accuracy when there’s a lot of non-text media in the posts / for different types of media? I’m wondering if a classifier like this does best when there’s a lot of text but gets confused when the post is predominantly something else? If errors are correlated with the type of media, that could affect your results.
\end{enumerate}

\subsubsection{Questions}

\begin{itemize}
    \item I didn’t know what telegram was until I looked it up, you may consider adding a little description of the platform
    \item Did your data collection violate Telegram’s terms of service? It seems like you had to do a lot to get around their site’s protections, so I’m a little concerned that they may not have wanted you to collect this data
    \item How could you tell if a user was a bot?
    \item Line 477: this is an association not causation right? Or have you proven causality?
    \item Can you explain in the text how to interpret Fig 5?
\end{itemize}


\begin{description}
    \item [Ethics Review Flag:] Yes
    \item[Ethics Review Description:] Are the terms of use violated in data collection? 
    \item [Scope:] 3 
    \item [Novelty:] 4
    \item [Technical Quality:] 4
    \item [Reviewer Confidence:] 3
\end{description}




\subsection{Reviewer r7nV}
\subsubsection{Review}
This contribution proposes a descriptive exploration of Telegram groups. The work is original and mostly clear. It is not always clear how the authors choose what to analyze and what not to analyze. However, it provides interesting statistics for people who would like to study Telegram, a platform that is still relatively understudied.

pros:

\begin{itemize}
    \item study of the "global" telegram ecosystem
    \item comprehensive and clear methodology
    \item study of an understudied dataset
    \item shed lights on the functioning of different types of telegram groups
    \item good ethical approach
\end{itemize}

cons:

\begin{itemize}
    \item motivation behind the directions of analysis could be better explained.
    \item channels are not studied at all
    \item some figures are difficult to read (e.g., Fig. 8)
    \item it seems that URL were not unshortened (bit.ly appears in Fig. 6), which potentially means that the domain ranking is wrong.
    \item no network study
\end{itemize}


\subsubsection{Questions}

Could you please clarify if you unshortened the URLs and respond to my above remarks.


\begin{description}
    \item [Ethics Review Flag:] No
    \item [Scope:] 3 
    \item [Novelty:] 5
    \item [Technical Quality:] 6
    \item [Reviewer Confidence:] 4
\end{description}


\subsection{Reviewer otNx}
\subsubsection{Review}

This paper presents a broad analysis across topics in Telegram. To do so, the work relies on a crawler to extract information from public Telegram groups (a code which is made open-source, and can be definitely beneficial to the community, as well as helps for reproducibility and to alleviate any possible ethical concerns).

The paper does not have a single aim or research question in place, but rather offers a broad analysis of different aspects, such as bots, language usage, video (both duration and also relevance in terms of video publication) and external links shared. As such, it is hard to assess the paper by general standards. Nonetheless, I believe the paper can provide a useful contribution to the community, and establishes an initial basis to perform more in-depth sociological studies. The current studies are relatively simple and more descriptive than anything else. At the end of each analysis, there is a ``main takeaways'' short paragraph offering the main insights. This is quite useful for the reader, however, the takeaways are not always grounded on evidence. One suggestion I would have for the paper would be to try and prove or provide quantitative evidence for each takeaway, which in the main comes from the main analysis but may require further analysis. For instance, in Section 4.2.1 the main takeaway starts with ``official bots’ impact on the activity of Telegram is significant''; Why is it ``significant''? What is the definition of significance used here? This could very well be a statistically-based research question which can be attempted to be answered based on data. I believe that complementing the descriptive analysis with more grounded insights can be beneficial.

While there are some ethical implications of this work, I haven't flagged it as I was not completely sure of the actual implications and the paper offers some clear explanation. The analysis is based on a crawler created to extract public topics from Telegram, at times possibly infringing some terms and conditions. The authors were up-front about this, and even contacted Telegram support, but they did not receive an answer. While I believe that the focus on public spaces and analytical nature (in which no personal information or even personal content is shared) make the work legit and ethical, I highlight it here as I’m not expert on the topic and the possible implications.
\subsubsection{Questions}

There are some comments of previous work focusing on textual content, but I believe these would differ from this study. Why wasn’t there more in-depth analysis of textual content? I believe this can complete this paper well.

How were the type of analysis decided? For instance, why focusing on the duration of videos and external links? Just want to know a bit more the rationale behind each analysis, as equally other types of analysis could have been done.

What is the evidence for each of the takeaways?



 
\begin{description}
    \item [Ethics Review Flag:] No
    \item [Scope:] 3 
    \item [Novelty:] 5
    \item [Technical Quality:] 5
    \item [Reviewer Confidence:] 2
\end{description}

\subsection{Reviewer vDWS}
\subsubsection{Review}
\subsubsection{Questions}

This paper offers a broad analysis of publicly accessible Telegram groups spanning multiple categories (from Education to Cryptos) through the proposal of an open-source tool to automate the collection of messages. The analysis is based on a starting dataset of 51.6M messages and 1.4M users, over a two-month period.

\textit{Strengths}

\begin{itemize}
    \item The topic-wise exploration might unveil more nuanced aspects that could have remained hidden in previous topic-specific or community-specific studies on Telegram.
    \item The proposed open-source tool represents a valuable contribution to the community interested in working with Telegram data.
    \item The unveiled findings contribute to shaping a fingerprint of the different topical communities present in Telegram.

\end{itemize}

\textit{Weaknesses}

\begin{itemize}

    \item While TGStat serves as a valuable aggregator for public Telegram channels, it can introduce bias in data collection as groups not cataloged by the service can remain underrepresented.
    \item Despite leading to a notable number of messages to analyze, the two-month data collection period can limit the generalizability of the reported findings, as long-term patterns (e.g., the impact of events on certain communities) cannot easily emerge in such a temporal window.
    \item Related to the previous point, given the "dynamic update" of data offered by the proposed tool, some temporal trend analysis (especially for the aspects in Sec. 4) would be appreciated.
    \item The scope of this manuscript seems to be primarily quantitative, yet complementing these findings with qualitative and more fine-grained aspects can strengthen the value of the work. For instance, within the Politics group, there can be different "subgroups" (e.g., from a specific political side) with a different impact on the unveiled patterns; similarly, one of these subgroups can be the one determining most of the trends the authors unveiled.
\end{itemize}


\begin{description}
    \item [Ethics Review Flag:] No
    \item [Scope:] 3 
    \item [Novelty:] 4
    \item [Technical Quality:] 3
    \item [Reviewer Confidence:] 3
\end{description}


\subsection{Reviewer 9fCp}
\subsubsection{Review}
This paper extensively analyzes public Telegram groups across varied topics, including Education, Erotic, Politics, and Cryptocurrencies. Utilizing an open-source crawler, the authors collect over 51 million messages across 669 groups, analyzing user interaction patterns, bot activity, language diversity, and multimedia usage. The study finds distinct communication behaviors based on topics, revealing both expected patterns (e.g., spam behavior) and novel insights (e.g., varying media sharing habits across groups).

Nice research methodologically with a large dataset on a platform we don’t hear much about. The paper is written and reads well. Its originality is high, as this paper addresses a gap in the literature on analyzing topic-based behavior on Telegram, a relatively underexplored platform. In terms of significance, the insights inform further studies on social media behavior and content moderation, although the results are not all that surprising.

So, on the plus side, a comprehensive data collection across multiple topics. Novel analysis of Telegram-specific user interactions and bot influence. There is a valuable open-source contribution through the crawler and dataset. For improvements, you should mention the ethical discussion around user tracking. There is a surface-level focus on bot behavior without delving deeply into user-only dynamics—no real comparison to existing social media research.

\subsubsection{Questions}

Major Issues: It is not clear what the research questions or objectives are. Is it to build and test a crawler? Or analysis of the topics collected? How do the results compare with prior studies on other social media platforms, especially concerning how Telegram usage may differ from or mirror platforms like WhatsApp or Facebook? Why so much focus on the bots? Seems like the user behavior would be more interesting. There is a lot of descriptive data, but it is not clear what to do with it. This is where some research questions (clearly stated) would help.


\begin{description}
    \item [Ethics Review Flag:] No
    \item [Scope:] 4 
    \item [Novelty:] 4
    \item [Technical Quality:] 6
    \item [Reviewer Confidence:] 3
\end{description}

\subsection{Paper metareview}
\subsubsection{Summary}

This paper presents a broad analysis of publicly accessible Telegram groups, examining user activity patterns across various topics, including Education, Erotic, Politics, and Cryptocurrencies. The authors developed an open-source tool to collect over 51 million messages from 669 Telegram groups. The study analyzes user interaction patterns, bot activity, language diversity, and multimedia usage, comparing these elements across different topic groups.

\subsubsection{Pros}
\begin{enumerate}
    \item \textbf{Novel exploration of an understudied platform}: Telegram's increasing popularity and unique features make it a relevant subject for study.
    \item \textbf{Comprehensive data collection and methodology}: The dataset of 51 million messages from 669 groups provides a substantial basis for analysis. The authors' methodology appears systematic and well-documented, covering various aspects of Telegram group activity.
    \item \textbf{Release of open-source crawler and dataset}: This contribution enables further research on Telegram by the broader scientific community.
    \item \textbf{Good ethical approach}: The authors considered ethical implications and adhered to Telegram's privacy policies during data collection. They also attempted to contact Telegram for this work.
\end{enumerate}

\subsubsection{Cons}
\begin{enumerate}
    \item \textbf{Lack of clear research questions and hypothesis}: The paper's goal is framed as a descriptive analysis, but the lack of specific research questions makes it difficult to assess the significance of the findings. While the authors clarified their aim as a descriptive analysis in their rebuttals, the paper currently lacks a clear framing of what it seeks to discover or test. One reviewer asked the authors to state the research questions, to which the authors replied, "How do users behave on Telegram groups in terms of the features they most often make use of to interact with others (e.g., video sharing, link sharing, use of reactions, polls, etc)? How do such platform usage patterns change across groups discussing different topics? What are the similarities and differences across topics?". The lack of subsequent discussion on these specific questions makes it difficult to assess their appropriateness or whether they accurately reflect the content and scope of the main text.
    \item \textbf{Limited generalizability due to sampling method}: The reliance on TGStat for group selection introduces potential bias, as groups not listed on the service are excluded. The authors acknowledge this limitation but explain that TGStat is suitable for their goal of providing a horizontal study across popular topics and groups.
    \item \textbf{Lack of discussion on the implications and importance of findings}: The paper primarily describes observed differences in non-text engagement across topics but does not adequately explain why these differences matter or what their practical implications are. The authors responded during the discussion by citing examples of how different media can reflect unique usage patterns.
    \item \textbf{Insufficient justification for analysis choices and limited exploration of textual content}: The justification behind the specific analyses needs to be clarified, and the paper could benefit from a more in-depth analysis of textual content. The authors responded that a full textual analysis is complex and beyond the scope of this paper.
    \item \textbf{Limited temporal scope}: The two-month data collection period may not capture long-term patterns or the impact of specific events on group dynamics. The authors acknowledge this limitation and suggest future work could explore the temporal dimension.
    \item \textbf{URL shortening and domain ranking}: Reviewer r7nV highlighted that URLs were not unshortened, potentially affecting the domain ranking analysis. In the rebuttal, the authors clarified that unshortening bit.ly URLs did not significantly change the domain ranking based on their data.
\end{enumerate}
\subsubsection{Overall Assessment}
This paper presents a valuable initial exploration of topic-wise differences in Telegram group activity, supported by a large dataset and a clear methodology. The release of the open-source crawler and dataset is a significant contribution to the research community. However, the paper's impact is currently limited by the lack of clearly defined research questions, a thorough discussion of the findings' implications, and a more robust justification for the chosen analyses. Also, the reliance on TGStat and the limited temporal scope also restrict the generalizability of the findings.



\section{Improvements}

Thanks to the reviewers' feedbacks, we introduced some minor improvements in our manuscript:

\begin{itemize}
    \item We include a brief description of Telegram and specified that Telegram includes one-to-one chats for those who are not aware of the platform features, as suggested by reviewer uQQ5;

    \item We better clarified motivations and research  questions, following the feedback of reviewers r7nV and 9fCp;
    
    \item We modified L477 to underline association rather than causality, following the suggestions of reviewer uQQ5;
    
    \item We modified the text to better describe Fig. 5, as pointed out by reviewer uQQ5;
    
    \item We introduced a short discussion about shortened URLs, according to what reviewer r7nV has pointed out;

    \item We better clarified the rational behind the analysis of the video size and duration and  and external links, following suggestions by reviewer otNx;
    
    \item We integrated numerical figures in subsection takeaways, following suggestions by reviewer otNx;

    \item We introduced some additional, minor tweaks to the text to respect The Web Conference's 8-pages limit after previous modifications.
    
\end{itemize}
